# Supplementary material for: Neural Image Re-Exposure
Source: arXiv:2305.13593 source file (2023-05-23)
Supplement: Supplementary file 1 [file supp.tex]

Remaining Problems:

1. \sout{Evaluate deblurring on real-captured data?} 

2. \sout{How to summarize the task? }Shutter related problems + Nerual Image Re-exposure

3. \sout{Should the introduction give so detailed description of the method?}

4. \sout{Another model name rather than SimXpo}  NIRE

\vspace{2em}
Terminology:

1. Neural Re-exposure:
\textbf{Re-exposure module}

2. visual content:
    visual content of the (captured) scene
    captured visual content

3. visual latent space:
project the visual content of the scene into the visual latent space;
\textbf{construction of visual latent space};

3. imaging effect
    bring different imaging effect

4. shutter strategy:
shutter-related problems;
shutter speed (slow/fast); 
shutter frequency; 
\sout{shutter timing};
shutter manner (timestamp, type, )
shutter timing?

\vspace{2em}
Core Expression:

1. In this work, we would like to explore a way for a more flexible \textit{re-exposure of a captured photo}

\clearpage
\appendix

\section*{Supplemental Material}

% 代码 with demo script
% a demo video
% TODO: 增加定性结果的方法比较：不用都跑，可以只跑几个，比如右边放两行，每行对应一个patch，放NAFNet, EDI, 另外一个eventbased的方法，EFNet, Ours,GT，一共6个
% TODO: 增加 RS -> GS blur 和 blur -> RS output的训练样本，做到更全面的reblur 
% TODO: 增加Attention和Decoder的结构细节
% TODO: A experiment on HQF
% 

Here you can include supplemental material that expands on the content in the main body of the document.

\subsection*{A.1 }

\subsection*{A.2 }
